# Supplementary material for: BandMaxSAT: A Local Search MaxSAT Solver with Multi-armed Bandit
Source: arXiv:2201.05544 source file (2022-06-16)
Supplement: Supplementary file 1 [file Appendix.tex]

\twocolumn[
\begin{@twocolumnfalse}
\section*{\centering{\LARGE{Appendix}}}
~\\
\end{@twocolumnfalse}
]

In the Appendix, we provide the detailed results of four solvers, PPMAB-c, SATLike-c, Loandra, and TT-Open-WBO-Inc (TT-OWI), that describe the distribution of scores per instances in each benchmark. The results of the (W)PMS instances from MSE2018, MSE2019, MSE2020, MSE2021 are shown in Figures \ref{fig-scores-18}, \ref{fig-scores-19}, \ref{fig-scores-20}, \ref{fig-scores-21}, respectively.
